# Supplementary material for: Efficiently parallelized modeling of tightly focused, large bandwidth laser pulses
Source: arXiv:1609.08146 ancillary file (2017-02-01)
Supplement: Supplementary file 1 [file SupplementalMaterial.pdf]

# Supplementary Material: Efficiently parallelized modeling of tightly focused, large bandwidth laser pulses

Joey Dumont,[1, *] Franois Fillion-Gourdeau,[1, 2] Catherine Lefebvre,[1, 2] Denis Gagnon,[1, 2] and Steve MacLean[1, 2, †]

[1] *Université du Québec, INRS-Énergie, Matériaux et Télécommunications, Varennes, Québec, Canada, J3X 1S2*

[2] *Institute for Quantum Computing, University of Waterloo, Waterloo, Ontario, Canada, N2L 3G1*

(Dated: November 29, 2016)

This supplemental material discusses the incident field models that were used in the numerical simulations of the main paper and provides explicit expressions of the Stratton-Chu integrals in cylindrical coordinates.

## I. FIELD MODELS

Using closed-form expressions to represent the incident field can be useful, even though the evaluation of Eqs. (11) of the main paper can be carried out for arbitrary incident fields. It allows for sampling the field at arbitrary points and eases the spectral normalization procedure. The following sections provide a derivation of the two beam models that were used in the numerical simulations presented in the main paper. The incident field models are solutions of the paraxial wave equation. This is a correct use of the approximation, as the incident field is assumed to be a highly collimated laser pulse. This assumption incurs an error on the order of the divergence angle, i.e. $\mathcal{O}(\epsilon)$, on the value of the incident field. Since Eqs. (11) of the main paper are linear in the fields, the resulting error in the reflected is $\mathcal{O}(\epsilon)$.

In this section, we give a brief overview of the paraxial wave equation and present two specific solutions, the Gaussian beam and the Gauss-Laguerre beam, which we use as a basis to represent any field configuration.

### A. Paraxial wave equation

In vacuum and in the Lorentz gauge, it can be shown that the electromagnetic vector potential $\boldsymbol{A}$, the scalar potential $\Phi$ and the electric field $\boldsymbol{E}$ all obey the same differential equation [1]

$$\left[\nabla^2 - \partial_{tt}\right]\{\boldsymbol{A}, \Phi, \boldsymbol{E}\} = 0, \tag{1}$$

where the Lorentz gauge is described by the relation

$$\nabla \cdot \boldsymbol{A} + \frac{\partial \Phi}{\partial t} = 0 \tag{2}$$

In the next sections, we will use the anstze

$$\boldsymbol{F} = \hat{\boldsymbol{a}}\psi(r,z)e^{-i\omega t - ikz} \tag{3a}$$

$$\Phi = \psi(r,z)e^{-i\omega t - ikz} \tag{3b}$$

where $\boldsymbol{F}$ is either $\boldsymbol{A}$ or $\boldsymbol{E}$ and $\hat{\boldsymbol{a}}$ is a constant unit vector. If we further make use of the paraxial approximation, Eq. (1) becomes [2, Eq. (2.11)]

$$\nabla_\perp^2\psi(r,z) - 2ik\partial_z\psi(r,z) = 0. \tag{4}$$

Choosing to use the anstze Eq. (3) for $\boldsymbol{A}$ with $\hat{\boldsymbol{a}} = \hat{\boldsymbol{z}}$ yields a radially polarized electromagnetic field. The field components can be obtained via the relations [3, Eq. (1.26)]

$$\boldsymbol{E} = ik\boldsymbol{A} + \frac{i}{k}\nabla(\nabla\cdot\boldsymbol{A}), \tag{5a}$$

$$\boldsymbol{B} = \nabla \times \mathbf{A}. \tag{5b}$$

where we used the Lorentz gauge condition (2) in Eq. (5a). Explicitly, the components read

$$E_r = \frac{i}{k}\partial_r\partial_z A_z, \tag{6a}$$

$$E_z = i\omega A_z + \frac{i}{k}\partial_z^2 A_z, \tag{6b}$$

$$B_\theta = -\partial_r A_z. \tag{6c}$$

Conversely, choosing to use the anstze for $\boldsymbol{F} = \boldsymbol{E}$ and $\hat{\boldsymbol{a}} = \hat{\boldsymbol{x}}$ yields an electric field polarized in the $\hat{\boldsymbol{x}}$. The associated magnetic field can be computed via Maxwell's equations.

In the following sections, we will present both radially polarized and linearly polarized paraxial solutions. Radially polarized beams have shown promise in multiple applications, such as direct electron acceleration [4].

### B. Gaussian Beams

The Gaussian beam is perhaps the most used model to describe laser light, as it describes well collimated beams [5].

*a. Radially polarized field* Analytical solutions of Eq. (4) for a radially polarized Gaussian beam have been derived by Salamin [6]. Specifically, we use the zeroth-

* Corresponding author: joey.dumont@gmail.com
† steve.maclean@emt.inrs.ca

order solution

$$E_r(r,\theta,z;k) = -E_0 \frac{2r}{kw_0^2} q^2 e^{-q\frac{r^2}{w_0^2} - ikz}, \tag{7a}$$

$$E_z(r,\theta,z;k) = iE_0 \frac{4}{k^2 w_0^2}\left[q^2 - q^3 \frac{r^2}{w_0^2}\right] e^{-q\frac{r^2}{w_0^2} - ikz}, \tag{7b}$$

$$B_\theta(r,\theta,z;k) = E_0 \frac{2r}{kw_0^2} q^2 e^{-q\frac{r^2}{w_0^2} - ikz}, \tag{7c}$$

where $q = i/(i - z/z_R)$ and $z_R = kw_0^2/2$ is the Rayleigh range of the beam. For highly collimated beams, $q \to 1$. The energy density is

$$\epsilon(k) = \frac{4\pi^2}{k^2}. \tag{7d}$$

*b. Linearly polarized field* In the linearly polarized case, the fields can be written directly as

$$E_x(r,z;k) = E_0 e^{-\frac{r^2}{w_0^2} - ikz}, \tag{8a}$$

$$B_y(r,z;k) = -E_0 e^{-\frac{r^2}{w_0^2} - ikz} \tag{8b}$$

where $E_0$ is an arbitrary normalization factor. The other components all vanish, i.e. $E_y = E_z = B_x = B_z = 0$. The energy density per mode is given by

$$\begin{aligned}\epsilon(k) &= 4\pi \oiint_A \mathrm{Re}\left\{\boldsymbol{f}_E^n n(\boldsymbol{r},k_n) \times \boldsymbol{f}_B^{n*}(\boldsymbol{r},k_n)\right\} \cdot d\boldsymbol{A}, \\ &= 2\pi^2 w_0^2. \end{aligned}\tag{8c}$$

### C. Gauss-Laguerre Fields

Another general solution of Eq. (4) is given by a sum of Gauss-Laguerre modes [7]

$$\psi(r,z) = \frac{w_0}{w(z)} \sum_{n=0}^{\infty} c_n L_n^{(0)}\left(\frac{2r^2}{w^2(z)}\right) \times e^{-\frac{r^2}{w^2(z)} - ik\frac{r^2}{2R(z)} + i\phi(z)}. \tag{9}$$

where $w(z) = w_0\sqrt{1 + (z/z_R)^2}$ is the beam waist, $R(z) = (z^2 + z_R^2)/z$ is the radius of curvature of the wavefront and $\phi(z) = \arctan(z/z_R)$ is the Gouy phase of Gaussian beams and where $L_n^{(0)}(x)$ is the associated Laguerre polynomial. It is defined by the power series [8, §22.3.9]

$$L_n^{(k)}(x) = \sum_{m=0}^{n} \frac{(-1)^m}{m!}\binom{n+k}{m+k} x^m. \tag{10}$$

When the field is collimated, the solution can be simplified to

$$\psi_n(r,z) = \sum_{n=0}^{\infty} c_n L_n^{(0)}\left(\frac{2r^2}{w_0^2}\right) e^{-\frac{r^2}{w_0^2}}. \tag{11}$$

*a. Radially Polarized Gauss-Laguerre Beams* The components of the radially polarized field can be obtained by evaluating the derivatives Eq. (6) of Eq. (9). To do so, we will need to use some properties of the generalized Laguerre polynomials, namely [8, §22.3.9, §22.7.31]

$$\frac{d^k}{dx^k} L_n^{(\alpha)}(x) = (-1)^k L_{n-k}^{(\alpha+k)}(x), \tag{12a}$$

$$L_{n-1}^{(1)}(x) = -L_n^{(0)}(x) + L_n^{(1)}(x). \tag{12b}$$

Evaluating this yields

$$E_r = -\frac{2r}{w_0^2} e^{-\frac{r^2}{w_0}} \sum_{n=0}^{N} c_n \left[2L_n^{(1)}\left(\frac{2r^2}{w_0^2}\right) - L_n^{(0)}\left(-\frac{2r^2}{w_0^2}\right)\right], \tag{13a}$$

$$E_z = 0, \tag{13b}$$

$$B_\theta = -E_r. \tag{13c}$$

To evaluate the energy density integral, it is useful write this expression as a polynomial. Using the definition (10), we can write the radial component as

$$E_r = -\frac{2r}{w_0^2} e^{-\frac{r^2}{w_0^2}} \sum_{n=0}^{N} c_n \sum_{k=0}^{n} \frac{(-1)^k}{k!}\binom{n}{k}\left[\frac{2n-k+1}{k+1}\right] x^k, \tag{14}$$

where $x = \frac{2r^2}{w_0^2}$. For later convenience, we define

$$B_k = \sum_{n=k}^{N} \frac{(-1)^k}{k!}\binom{n}{k}\left[\frac{2n-k+1}{k+1}\right]. \tag{15}$$

Recall that for a radially polarized beam, the Poynting vector is simply $\boldsymbol{S} = E_r^2 \hat{\boldsymbol{z}}$. We must evaluate the square of the radial component:

$$\begin{aligned} E_r^2 &= \left(\frac{2r}{w_0^2}\right)^2 e^{-\frac{2r^2}{w_0^2}} \sum_{k_1=0}^{N}\sum_{k_2=0}^{N} B_{k_1} B_{k_2} x^{k_1+k_2}, \\ &= \frac{2r}{w_0^2} e^{-\frac{r^2}{w_0^2}} \sum_{k=0}^{2N} C_k x^k, \end{aligned}\tag{16}$$

where

$$\begin{aligned} C_k &= \sum_{l=0}^{k} B_l B_{k-l}, \\ &= \frac{(-1)^k}{k!} \sum_{l=0}^{k}\sum_{n_1=l}^{N}\sum_{n_2=k-l}^{N} c_{n_1} c_{n_2}\binom{k}{l}\binom{n_1}{l}\binom{n_2}{k-l} \\ &\times \left[\frac{2n_1 - k + 1}{l+1}\right]\left[\frac{2n_2 - (k-l) + 1}{k-l+1}\right]. \end{aligned}\tag{17}$$

The integral reduces to a polynomial times a Gaussian function. This can readily be integrated to yield [9, §3.381.11]

$$\epsilon(k) = \pi \sum_{k=0}^{2N} C_k (k+1)!. \tag{18}$$

*b. Linearly Polarized Gauss-Laguerre Beams* Since the vector potential and the electric field obey mathematically equivalent differential equations, then both fields admit the same solutions. We can then directly write the solutions for a collimated field as

$$E_x(r,z) = e^{-\frac{r^2}{w_0^2}} \sum_{n=0}^{\infty} c_n L_n^{(0)}\left(\frac{2r^2}{w_0^2}\right), \tag{19a}$$

$$B_y(r,z) = -E_x. \tag{19b}$$

To evaluate the energy density, we repeat the same steps as for the radially polarized case. The series coefficients now read

$$B_k = \sum_{n=k}^{N} c_n \frac{(-1)^k}{k!}\binom{n}{k}, \tag{20a}$$

$$C_k = \frac{(-1)^k}{k!}\sum_{l=0}^{k}\sum_{n_1=l}^{N}\sum_{n_2=k-l}^{N} c_{n_1}c_{n_2}\binom{k}{l}\binom{n_1}{l}\binom{n_2}{k-l}. \tag{20b}$$

The energy density is then

$$\epsilon(k) = \frac{\pi w_0^2}{2}\sum_{k=0}^{2N} C_k k!. \tag{21}$$

## II. EXPLICIT FORMULAE FOR THE STRATTON-CHU REPRESENTATION

In this section, we provide some explicit expressions of Eqs. (11) of the main paper in cylindrical coordinates. We consider only the case where the mirror $S$ has an explicit parametrization of the form $z = F(r,\theta)$. The normal to this surface takes the form

$$\begin{aligned}\hat{\boldsymbol{n}} &= \frac{\nabla\left[z - F(r,\theta)\right]}{\left|\nabla\left[z - F(r,\theta)\right]\right|}, \\ &= \frac{-\partial_r F\hat{\boldsymbol{r}} - \frac{1}{r}\partial_\theta F\hat{\boldsymbol{\theta}} + \hat{\boldsymbol{z}}}{\sqrt{\left(\partial_r F\right)^2 + \left(\frac{1}{r}\partial_\theta F\right)^2 + 1}}, \qquad (22a)\\ &= \frac{\boldsymbol{N}}{\sqrt{\left(\partial_r F\right)^2 + \left(\frac{1}{r}\partial_\theta F\right)^2 + 1}}, \qquad (22b)\end{aligned}$$

while the surface element, or Jacobian, is

$$dS = r dr d\theta\sqrt{\left(\partial_r F\right)^2 + \left(\frac{1}{r}\partial_\theta F\right)^2 + 1}. \tag{23}$$

In the Stratton-Chu equations, the square root factors coming from the normal and the Jacobian will cancel, leaving only the cylindrical coordinates $r$ factor. The Green's function can be expressed as

$$g = \frac{e^{-iku}}{4\pi u} \tag{24a}$$

where

$$u = \sqrt{r'^2 + r^2 - 2rr'\cos(\theta' - \theta) + (z' - F(r,\theta))^2} \tag{24b}$$

and its gradient is

$$\begin{aligned}\nabla g &= \left[\frac{ik}{u} - \frac{1}{u^2}\right]\Big\{\left(r\cos(\theta-\theta') - r'\right)\hat{\boldsymbol{r}} + r\sin(\theta-\theta')\hat{\boldsymbol{\theta}} \\ &\qquad + \left(F(r,\theta) - z'\right)\hat{\boldsymbol{z}}\Big\} g, \qquad (24c)\\ &= \boldsymbol{G} g. \qquad (24d)\end{aligned}$$

Substituting this into Eqs. (11) of the main paper yields

$$\begin{aligned}\boldsymbol{E}_{\text{ref}}(\boldsymbol{r}',k) &= 2\int_S \left\{ik(\boldsymbol{N}\times\boldsymbol{B}_{\text{inc}}) + (\boldsymbol{N}\cdot\boldsymbol{E}_{\text{inc}})\boldsymbol{G}\right\} g\, r dr d\theta \\ &\quad - \frac{2}{ik}\oint_{\partial S} g\mathbf{G}\left[\hat{\boldsymbol{n}}\times(\hat{\boldsymbol{n}}\times\boldsymbol{B}_{\text{inc}})\right]\cdot d\boldsymbol{\ell}, \qquad (25a)\end{aligned}$$

$$\boldsymbol{B}_{\text{ref}}(\boldsymbol{r}',k) = 2\int_S \left\{(\boldsymbol{N}\times\boldsymbol{B}_{\text{inc}})\times\boldsymbol{G}\right\} G r dr d\theta. \tag{25b}$$

The parabolic mirror is defined by

$$z = \frac{r^2}{4f} - f \tag{26}$$

and its normal is

$$\hat{\boldsymbol{n}} = \frac{-r\hat{\boldsymbol{r}} + 2f\hat{\boldsymbol{z}}}{\sqrt{r^2 + 4f^2}}. \tag{27}$$

For this type of mirror, the Stratton-Chu equations can be written explicitly as

$$
\begin{aligned}
E_r(\boldsymbol{r}',k) = 2\int_0^{r_{\max}}\int_0^{2\pi} \Bigg\{ ik \left[\left(\frac{r}{2f}B_{\mathrm{inc},z} + B_{\mathrm{inc},r}\right)\sin(\theta'-\theta) - B_{\mathrm{inc},\theta}\cos(\theta'-\theta)\right] \\
- \left[\frac{1-iku}{u^2}\right]\left[r\cos(\theta-\theta') - r'\right]\left[E_{\mathrm{inc},z} - \frac{r}{2f}E_{\mathrm{inc},r}\right]\Bigg\} grdrd\theta \\
+ \frac{2r_{\max}}{ik}\int_0^{2\pi}\frac{iku-1}{u^2} g\left[r_{\max}\cos(\theta-\theta') - r')\right] B_{\mathrm{inc},\theta}d\theta, \qquad (28a)
\end{aligned}
$$

$$
\begin{aligned}
E_\theta(\boldsymbol{r},t) = 2\int_0^{r_{\max}}\int_0^{2\pi} \Bigg\{ ik \left[\left(\frac{r}{2f}B_{\mathrm{inc},z} + B_{\mathrm{inc},r}\right)\cos(\theta'-\theta) - B_{\mathrm{inc},\theta}\sin(\theta'-\theta)\right] \\
- \left[\frac{1-iku}{u^2}\right]\left[r\sin(\theta-\theta')\right]\left[E_{\mathrm{inc},z} - \frac{r}{2f}E_{\mathrm{inc},r}\right]\Bigg\} grdrd\theta + 2\frac{r_{\max}^2}{ik}\int_0^{2\pi}\left[\frac{iku-1}{u^2}\right]\sin(\theta-\theta')B_{\mathrm{inc},\theta}d\theta, \qquad (28b)
\end{aligned}
$$

$$
\begin{aligned}
E_z(\boldsymbol{r}',k) = 2\int_0^{r_{\max}}\int_0^{2\pi} \left\{ -ik\frac{r}{2f}B_{\mathrm{inc},\theta} - \left[\frac{1-iku}{u^2}\right]\left[z-z'\right]\left[E_{\mathrm{inc},z} - \frac{r}{2f}E_{\mathrm{inc},r}\right]\right\} Grdrd\theta \\
+ \frac{2r_{\max}}{ik}\int_0^{2\pi}\left[ik - \frac{1}{u}\right]\frac{e^{iku}}{u^2}\left[z-z'\right]B_{\mathrm{inc},\theta}d\theta, \qquad (28c)
\end{aligned}
$$

$$
\begin{aligned}
B_r(\boldsymbol{r}',k) = -2\int_0^{r_{\max}}\int_0^{2\pi}\left[\frac{1-iku}{u^2}\right] g\Bigg\{\left(-\frac{r^2}{2f} + (z-z')\right)B_{\mathrm{inc},\theta}\sin(\theta'-\theta) \\
+ \left(\frac{r}{2f}B_{\mathrm{inc},z} + B_{\mathrm{inc},r}\right)(z-z')\cos(\theta-\theta_{\mathcal{S}})\Bigg\} rdrd\theta, \qquad (28d)
\end{aligned}
$$

$$
B_\theta(\boldsymbol{r}',k) = 2\int_0^{r_{\max}}\int_0^{2\pi}\left[ik - \frac{1}{u}\right]\frac{e^{iku}}{u^2}\left\{\frac{r}{2f}(r' - r\cos\theta) - (z-z')\right\} B_{\mathrm{inc},\theta}rdrd\theta, \qquad (28e)
$$

$$
\begin{aligned}
B_z(\boldsymbol{r},t) = -2\int_0^{r_{\max}}\int_0^{2\pi}\left[\frac{1-iku}{u^2}\right] g\Bigg\{\left(-\frac{r^2}{2f} + (z-z')\right)B_{\mathrm{inc},\theta}\sin(\theta'-\theta) \\
+ \left(\frac{r}{2f}B_{\mathrm{inc},z} + B_{\mathrm{inc},r}\right)(z-z')\cos(\theta-\theta)\Bigg\} rdrd\theta. \qquad (28f)
\end{aligned}
$$


[1] Y. I. Salamin, Phys. Rev. A **92**, 063818 (2015).
[2] M. Lax, W. H. Louisell, and W. B. McKnight, Phys. Rev. A **11**, 1365 (1975).
[3] J. A. Stratton, *Electromagnetic Theory* (McGraw-Hill, 1941).
[4] C. Varin, S. Payeur, V. Marceau, S. Fourmaux, A. April, B. Schmidt, P.-L. Fortin, N. Thiré, T. Brabec, F. Légaré, J.-C. Kieffer, and M. Piché, Appl. Sci. **3**, 70 (2013).
[5] A. E. Siegman, *Lasers* (University Science Books, Mill Valley, 1986) p. 1304.
[6] Y. I. Salamin, New J. Phys. **8**, 133 (2006).
[7] L. Allen, M. W. Beijersbergen, R. J. C. Spreeuw, and J. P. Woerdman, Phys. Rev. A **45**, 8185 (1992).
[8] M. Abramowitz and I. A. Stegun, *Handbook of Mathematical Functions* (Dover Publications, 1965).
[9] I. S. Gradshteyn and I. M. Ryzhik, *Table of Integrals, Series, and Products*, 7th ed. (Academic Press, 2007).
